# Supplementary material for: Beyond the standard quantum limit of parametric amplification
Source: arXiv:2011.00914 ancillary file (2020-11-11)
Supplement: Supplementary file 1 [file Supplementary_Material.pdf]

# Supplementary material for the paper “Beyond the standard quantum limit of parametric amplification”

Michael Renger<sup>1,2,\*</sup>, S. Pogorzalek<sup>1,2</sup>, Q. Chen<sup>1,2</sup>, Y. Nojiri<sup>1,2</sup>, K. Inomata<sup>4,5</sup>, Y. Nakamura<sup>4,6</sup>,

M. Partanen<sup>1</sup>, A. Marx<sup>1</sup>, R. Gross<sup>1,2,3</sup>, F. Deppe<sup>1,2,3</sup>, and K. G. Fedorov<sup>1,2†</sup>

<sup>1</sup> *Walther-Meißner-Institut, Bayerische Akademie der Wissenschaften, D-85748 Garching, Germany*

<sup>2</sup> *Physik-Department, Technische Universität München, D-85748 Garching, Germany*

<sup>3</sup> *Munich Center for Quantum Science and Technology (MCQST), Schellingstr. 4, 80799 Munich, Germany*

<sup>4</sup> *RIKEN Center for Emergent Matter Science (CEMS), Wako, Saitama 351-0198, Japan*

<sup>5</sup> *National Institute of Advanced Industrial Science and Technology,  
1-1-1 Umezono, Tsukuba, Ibaraki, 305-8563, Japan*

<sup>6</sup> *Research Center for Advanced Science and Technology (RCAST),  
The University of Tokyo, Meguro-ku, Tokyo 153-8904, Japan*

(Dated: November 11, 2020)

# QUANTUM LIMITS FOR NARROWBAND AND BROADBAND AMPLIFICATION

We start from Eq. (5) in the main text

$$\hat{c}(\omega) = \int_{\mathcal{I}} d\tilde{\omega} [M(\omega, \tilde{\omega})\hat{a}(\tilde{\omega}) + L(\omega, \tilde{\omega})\hat{a}^\dagger(\tilde{\omega})] + \hat{f}(\omega), \quad (\text{S1})$$

where  $\hat{c}(\omega)$  denotes the amplified output mode,  $\hat{a}(\tilde{\omega})$  denotes an input mode at frequency  $\tilde{\omega}$  which is amplified with gain  $M(\omega, \tilde{\omega})$ , and  $\hat{a}^\dagger(\tilde{\omega})$  is a phase-conjugated input mode which is amplified with signal gain  $L(\omega, \tilde{\omega})$  [S1]. The bosonic mode  $\hat{f}(\omega)$  represents the noise added by the amplifier, referred to the amplifier output, and guarantees that the output as well as the input modes fulfill the continuum bosonic commutation relations

$$[\hat{a}(\omega), \hat{a}^\dagger(\omega')] = 2\pi\delta(\omega - \omega'), \quad [\hat{a}(\omega), \hat{a}(\omega')] = 0, \quad (\text{S2})$$

$$[\hat{c}(\omega), \hat{c}^\dagger(\omega')] = 2\pi\delta(\omega - \omega'), \quad [\hat{c}(\omega), \hat{c}(\omega')] = 0 \quad (\text{S3})$$

which have to be satisfied by the bosonic operators  $\hat{a}(\omega)$  and  $\hat{c}(\omega)$ . In a parametric amplification process, every input mode  $\hat{a}(\tilde{\omega})$  can be associated with a corresponding phase-conjugated idler mode at frequency  $\tilde{\omega}_i = 2\omega_0 - \tilde{\omega}$  [S2], where  $\omega_0$  is the center frequency of the parametric gain function. For the output mode at frequency  $\omega$ , we hence have

$$M(\omega, \tilde{\omega}) = M(\tilde{\omega})\delta(\omega - \tilde{\omega}) \quad L(\omega, \tilde{\omega}) = L(\tilde{\omega}_i)\delta(\omega - \tilde{\omega}_i). \quad (\text{S4})$$

We assume that the input signal is centered around the reconstruction frequency  $\omega_s$  with a single-sided bandwidth  $b_s$  (total bandwidth  $2b_s$ ). Hence, Eq. (S1) gives

$$\hat{c}(\omega) = \int_{\omega_s - b_s}^{\omega_s + b_s} d\tilde{\omega} [M(\tilde{\omega})\delta(\omega - \tilde{\omega})\hat{a}(\tilde{\omega}) + L(\tilde{\omega}_i)\delta(\omega - \tilde{\omega}_i)\hat{a}^\dagger(\tilde{\omega})] + \hat{f}(\omega). \quad (\text{S5})$$

We use the relation

$$\int_a^b g(x)\delta(x)dx = g(0)\mathbb{1}[a, b](0) \quad (\text{S6})$$

for any function  $g$ , where

$$\mathbb{1}[a, b](x) = \begin{cases} 1 & a \leq x \leq b \\ 0 & \text{else} \end{cases}. \quad (\text{S7})$$

We obtain

$$\hat{c}(\omega) = M(\omega)\mathbb{1}_s(\omega)\hat{a}(\omega) + L(\omega_i)\mathbb{1}_i(\omega)\hat{a}^\dagger(\omega_i) + \hat{f}(\omega), \quad (\text{S8})$$

with  $\omega_i = 2\omega_0 - \omega$  and

$$\mathbb{1}_s(\omega) \equiv \mathbb{1}[\omega_s - b_s, \omega_s + b_s](\omega) = \Theta(\omega - \omega_s + b_s) - \Theta(\omega - \omega_s - b_s), \quad (\text{S9})$$

$$\mathbb{1}_i(\omega) \equiv \mathbb{1}[2\omega_0 - \omega_s - b_s, 2\omega_0 - \omega_s + b_s](\omega) = \Theta(\omega - 2\omega_0 + \omega_s + b_s) - \Theta(\omega - 2\omega_0 + \omega_s - b_s), \quad (\text{S10})$$

where  $\Theta$  is the Heaviside step function. We calculate the commutators

$$\begin{aligned} [\hat{c}(\omega), \hat{c}^\dagger(\omega')] &= M(\omega)M^*(\omega')\mathbb{1}_s(\omega)\mathbb{1}_s(\omega')[\hat{a}(\omega), \hat{a}^\dagger(\omega')] \\ &\quad - L(\omega_i)L^*(\omega'_i)\mathbb{1}_i(\omega)\mathbb{1}_i(\omega')[\hat{a}(\omega'_i), \hat{a}^\dagger(\omega_i)] + [\hat{f}(\omega), \hat{f}^\dagger(\omega')], \end{aligned} \quad (\text{S11})$$

which results in

$$[\hat{f}(\omega), \hat{f}^\dagger(\omega')] = 2\pi\delta(\omega - \omega')(1 - M(\omega)M^*(\omega')\mathbb{1}_s(\omega)\mathbb{1}_s(\omega') + L(\omega_i)L^*(\omega'_i)\mathbb{1}_i(\omega)\mathbb{1}_i(\omega')). \quad (\text{S12})$$

For the symmetrized fluctuations of the additive noise operator  $\hat{f}(\omega)$ , we find

$$\langle |\Delta \hat{f}|^2 \rangle \equiv \frac{1}{2} \langle \hat{f}(\omega)\hat{f}^\dagger(\omega') + \hat{f}^\dagger(\omega')\hat{f}(\omega) \rangle - \underbrace{\langle \hat{f}(\omega) \rangle \langle \hat{f}^\dagger(\omega') \rangle}_{=0} = 2\pi G_n(\omega)S_f(\omega)\delta(\omega - \omega'), \quad (\text{S13})$$

where  $G_n(\omega)$  is the parametric gain and  $S_f(\omega)$  is the noise power spectral density in units of photons per bandwidth. In Eq. (S13), we assumed that the expectation value of the fluctuations vanishes. We use the Heisenberg uncertainty principle  $\langle |\Delta \hat{f}|^2 \rangle \geq 1/2 \langle [\hat{f}(\omega), \hat{f}^\dagger(\omega')] \rangle$  and integrate over  $\omega'$

$$S_f(\omega) \geq \frac{1}{2G_n(\omega)} |1 - |M(\omega)|^2 \mathbb{1}_s(\omega) + |L(\omega_i)|^2 \mathbb{1}_i(\omega)|. \quad (\text{S14})$$

The quantities  $M(\omega)$  and  $L(\omega_i)$  are related to  $G_n(\omega)$  via  $|M(\omega)|^2 = G_n(\omega)$  and  $|L(\omega_i)|^2 = G_n(\omega) - 1$ , which yields

$$S_f(\omega) \geq \frac{1}{2G_n(\omega)} |\mathbb{1}_i(\omega) - 1 + G_n(\omega)(\mathbb{1}_s(\omega) - \mathbb{1}_i(\omega))|. \quad (\text{S15})$$

We get the number of added noise photons  $n_f$ , added by the mode  $\hat{f}(\omega)$ , by integrating Eq. (S15) over all output mode frequencies  $[\omega_s - \gamma, \omega_s + \gamma]$ . The output mode bandwidth  $\gamma$  is limited by the single-sided measurement bandwidth  $B$

$$\gamma = \begin{cases} b_s & b_s \leq B \\ B & \text{else} \end{cases}. \quad (\text{S16})$$

We obtain

$$\int_{\omega_s - \gamma}^{\omega_s + \gamma} S_f(\omega) d\omega = 2\gamma n_f \geq \frac{1}{2} \int_{\omega_s - \gamma}^{\omega_s + \gamma} (\mathbb{1}_s(\omega) - \mathbb{1}_i(\omega)) d\omega + \frac{1}{2} \int_{\omega_s - \gamma}^{\omega_s + \gamma} \frac{1}{G_n(\omega)} (\mathbb{1}_i(\omega) - 1) d\omega. \quad (\text{S17})$$

Equation (S17) gives the general constraint on the added noise, depending on the bandwidth of the signal. For  $b_s \leq b_1 = 2\Delta - B$ , we have  $\mathbb{1}_i(\omega) = 0$ , whereas for  $b_s \geq b_2 = 2\Delta + B$ , we always find  $\mathbb{1}_i(\omega) = 1$ , resulting in  $n_f \geq 0$ .

*Recovering the standard quantum limit* For narrowband signals at  $\omega_s$ , we assume  $b_s \ll B$  and hence  $\gamma = b_s$ . We assume a frequency independent gain within the signal bandwidth  $G_n(\omega) = G(\omega) \simeq G_n(\omega_s) \equiv G_n$ . Furthermore, we have  $\mathbb{1}_i(\omega) = 0$  and  $\mathbb{1}_s(\omega) = 1$ . Thus, we find

$$2b_s n_f \geq \frac{1}{2} \int_{\omega_s - b_s}^{\omega_s + b_s} \left(1 - \frac{1}{G_n}\right) d\omega \simeq \frac{1}{2} \left(1 - \frac{1}{G_n}\right) \cdot 2b_s \quad (\text{S18})$$

which reproduces the standard quantum limit (SQL) for narrowband signals.

*General Solution for Lorentzian Gain Function* We rewrite Eq. (S17) as

$$n_f \geq \frac{1}{4\gamma} \int_{\omega_s - \gamma}^{\omega_s + \gamma} \left(1 - \frac{1}{G_n(\omega)}\right) d\omega + \frac{1}{4\gamma} \int_{\mathcal{I}_i} \mathbb{1}_i(\omega) \left(\frac{1}{G_n(\omega)} - 1\right) d\omega, \quad (\text{S19})$$

where  $\mathcal{I}_i$  is the set of all input signal modes which overlap with the idler sideband measurement bandwidth. We find

$$\mathcal{I}_i = [2\Delta + \omega_s - b_s, 2\Delta + \omega_s + b_s] \cap [\omega_s - B, \omega_s + B] = [\max(2\Delta + \omega_s - b_s, \omega_s - B), \min(2\Delta + \omega_s + b_s, \omega_s + B)]. \quad (\text{S20})$$

We need to distinguish between the four cases  $b_s \leq B$ ,  $B \leq b_s \leq b_1$ ,  $b_1 \leq b_s \leq b_2$  and  $b_s \geq b_2$ . For  $\mathcal{I}_i$ , we find

$$\mathcal{I}_i = \begin{cases} \emptyset & b_s \leq B, \\ \emptyset & B \leq b_s \leq b_1, \\ [2\Delta + \omega_s - b_s, \omega_s + B] & b_1 \leq b_s \leq b_2, \\ [\omega_s - B, \omega_s + B] & b_s \geq b_2. \end{cases} \quad (\text{S21})$$

We describe the JPA gain curve as a Lorentzian centered at  $\omega_0$  with half-width-half-maximum bandwidth  $b_J$  [S3, S4].

$$G_n(\omega) = 1 + \frac{G_0 b_J^2}{b_J^2 + (\omega - \omega_0)^2}. \quad (\text{S22})$$

In the first case, we have  $b_s \leq B$ , which implies  $\gamma = b_s$ , according to Eq. (S16). We find

$$2b_s n_f \geq \frac{1}{2} \int_{\omega_s - b_s}^{\omega_s + b_s} \left(1 - \frac{1}{G_n(\omega)}\right) d\omega = \frac{G_0}{2(G_0 + 1)} \int_{\omega_s - b_s}^{\omega_s + b_s} \frac{1}{1 + \left(\frac{\omega - \omega_0}{b\sqrt{G_0 + 1}}\right)^2} d\omega. \quad (\text{S23})$$

Evaluating the integral yields

$$n_f \geq \frac{G_0 b_J}{4b_s \sqrt{G_0 + 1}} \arctan \left( \frac{2b_s b_J \sqrt{G_0 + 1}}{b_J^2 (G_0 + 1) + \Delta^2 - b_s^2} \right). \quad (\text{S24})$$

We define the gain-bandwidth product as  $\tau = b_J \sqrt{G_0}$  and approximate  $G_0 + 1 \simeq G_0$ , since  $G_0 \gg 1$  [S5]. Thus, we obtain

$$n \geq \frac{1}{4\beta_s} \arctan \left( \frac{2\beta_s}{1 + \delta^2 - \beta_s^2} \right), \quad (\text{S25})$$

where  $\beta_s \equiv b_s/\tau$ ,  $\beta \equiv B/\tau$  and  $\delta \equiv \Delta/\tau$ . In our experiment, we have  $\tau \simeq 20$  MHz,  $\Delta \simeq 0.3$  MHz,  $B \simeq 0.2$  MHz and find [S5]

$$n_f \geq \frac{1}{2} \frac{1}{1 + \delta^2} + \mathcal{O}(\beta_s^2) = 0.4999 \simeq \frac{1}{2}. \quad (\text{S26})$$

As a result, the Lorentzian shape of the gain curve only implies a small correction to the SQL of 1/2 in the narrowband case  $\beta_s \ll 1$ .

For the second case, we obtain  $\gamma = B$ . Thus, we need to solve

$$2Bn_f \geq \frac{1}{2} \int_{\omega_s - B}^{\omega_s + B} \left( 1 - \frac{1}{G_n(\omega)} \right) d\omega. \quad (\text{S27})$$

A similar calculation as in the first case gives

$$n_f \geq \frac{1}{4\beta} \arctan \left( \frac{2\beta}{1 + \delta^2 - \beta^2} \right), \quad (\text{S28})$$

where  $\beta \equiv B/\tau$  and  $G_0 \simeq G_0 + 1$ .

In the third case,  $b_1 \leq b_s \leq b_2$ , we have

$$2Bn_f \geq \frac{1}{2} \int_{\omega_s - B}^{\omega_s + B} \left( 1 - \frac{1}{G_n(\omega)} \right) d\omega + \frac{1}{2} \int_{2\Delta + \omega_s - b_s}^{\omega_s + B} \left( \frac{1}{G_n(\omega)} - 1 \right) d\omega = \frac{1}{2} \int_{\omega_s - B}^{2\Delta + \omega_s - b_s} \left( 1 - \frac{1}{G_n(\omega)} \right) d\omega, \quad (\text{S29})$$

which yields

$$n_f \geq \frac{1}{4\beta} \arctan \left( \frac{2(\delta + \beta - \beta_s)}{1 + \beta\beta_s + \delta(\beta_s - \beta) - \delta^2} \right). \quad (\text{S30})$$

In the fourth case, we immediately obtain

$$2Bn_f \geq \int_{\omega_s - B}^{\omega_s + B} \left( 1 - \frac{1}{G_n(\omega)} \right) d\omega + \frac{1}{2} \int_{\omega_s - B}^{\omega_s + B} \left( \frac{1}{G_n(\omega)} - 1 \right) d\omega = 0. \quad (\text{S31})$$

## JPA SAMPLES

The Josephson parametric amplifiers (JPAs) [S3] used in our experiment were designed and manufactured at NEC Smart Energy Research Laboratories, Japan and RIKEN, Japan. Each JPA consists of a  $\lambda/4$ -superconducting microwave resonator in a coplanar waveguide geometry. The resonator is short-circuited to the ground plane via a direct current superconducting quantum interference device (dc-SQUID) [S6]. A 300  $\mu\text{m}$  thick silicon chip, covered by a thermal oxide, is used for the substrate. The resonator and the pump line are patterned into a 50 nm thick sputtered Nb film. An aluminum shadow evaporation technique is used to fabricate the dc-SQUID. The resonant frequency  $\omega_0$  of the JPA can be tuned statically by an external coil or dynamically by a microwave signal applied via an on-chip antenna (pump line). In order to realize nondegenerate amplification, a strong coherent pump signal at  $\omega_p = 2\omega_0$  is applied, and the resonant frequency  $\omega_0$  is detuned by  $\Delta$  from the signal reconstruction frequency  $\omega_s$ . For each JPA, a commercial circulator is used to separate incoming from outgoing signals. In Tab.S1, we summarize the device parameters for our JPAs, which are determined by spectroscopic measurements [S6].

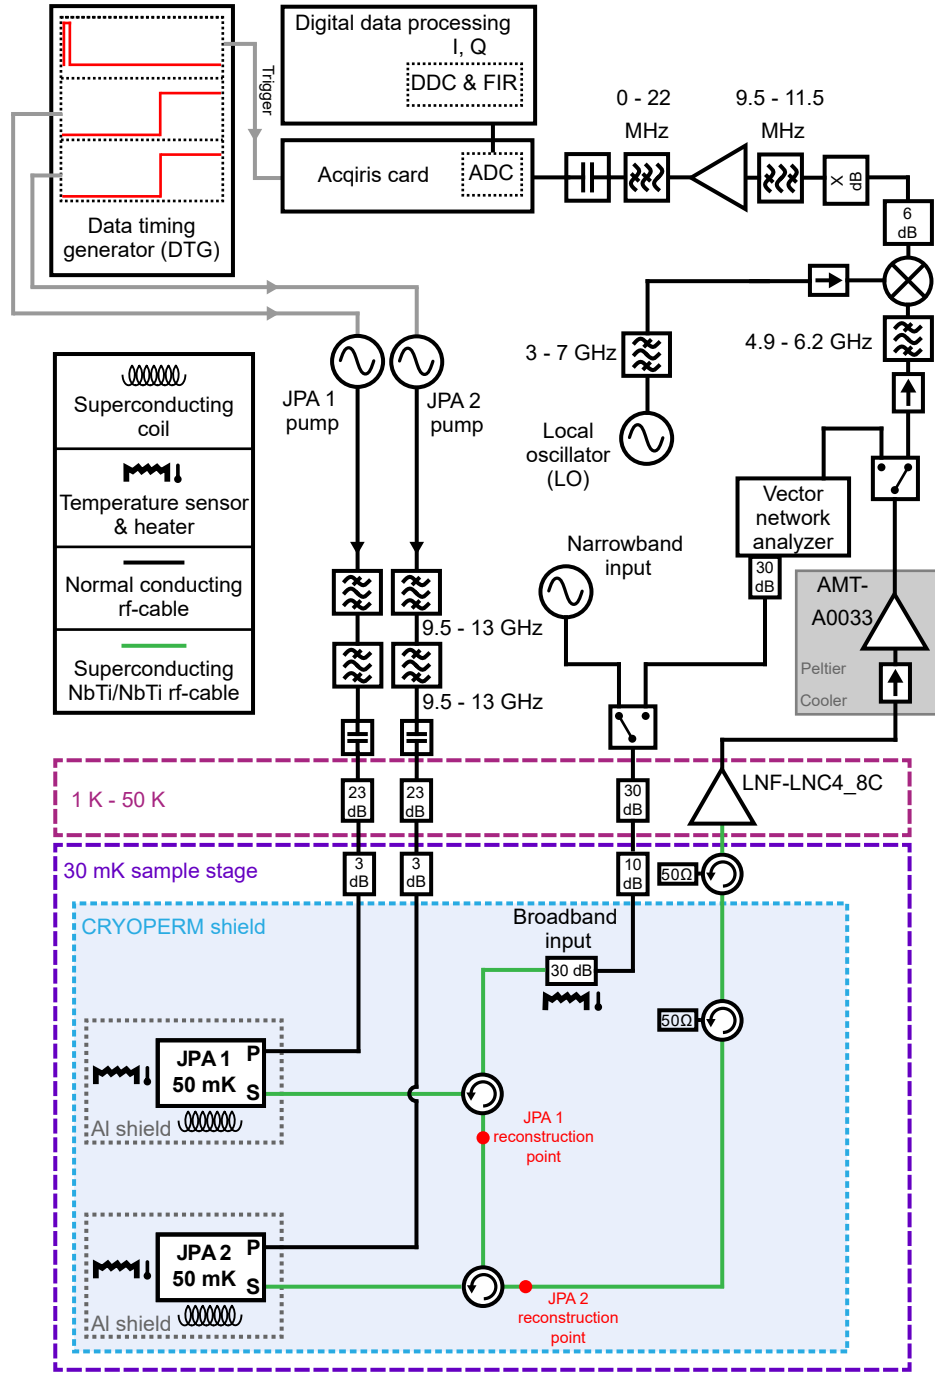

Figure S1. Experimental scheme and digital data processing setup for the quantum efficiency measurements. The output signal is amplified in multiple stages, down-converted and digitized. The measurement bandwidth  $B$  is determined by the finite-impulse response (FIR) filter. A data timing generator (DTG) enables pulsed measurements, which is necessary for the reference-state reconstruction.

## EXPERIMENTAL SETUP

The cryogenic setup as well as the room temperature electronics for data acquisition and digital signal processing are shown in Fig. S1. Both JPAs are temperature stabilized at 50 mK, which suppresses noise and gain variations caused by fluctuations of the JPA temperature. During the measurement with only JPA 1 (JPA 2), the resonant frequency

Table S1. JPA Parameters extracted by fitting the dependence of the resonant frequency  $\omega_0/2\pi$  of the JPAs on the applied magnetic flux [S6]. Here,  $I_c$  is the critical current and  $E_J = I_c \Phi_0/2\pi$  is the coupling energy of a e Josephson junction.  $L_{\text{loop}}$  and  $\beta_L = 2L_{\text{loop}}I_c/\Phi_0$  are the loop inductance and screening parameter of the dc-SQUID, respectively. The frequency of the bare resonator is denoted by  $\omega_r/2\pi$ . The Josephson junctions of the dc-SQUID are assumed to be identical. The external quality factors  $Q_{\text{ext}}$  and internal quality factors  $Q_{\text{int}}$  are obtained from independent fits of the JPA spectral linewidths [S6].

| Sample | $I_c$ ( $\mu\text{A}$ ) | $\beta_L$ | $L_{\text{loop}}$ (pH) | $\omega_r/2\pi$ (GHz) | $E_J/h$ (THz) | $Q_{\text{ext}}$ | $Q_{\text{int}}$ |
|--------|-------------------------|-----------|------------------------|-----------------------|---------------|------------------|------------------|
| JPA 1  | 2.45                    | 0.09      | 35.8                   | 5.808                 | 1.22          | 300–360          | >30000           |
| JPA 2  | 2.41                    | 0.10      | 40.7                   | 5.838                 | 1.20          | 240–260          | >30000           |

of JPA 2 (JPA 1) is far detuned from the signal reconstruction frequency  $\omega_s$  via a dc-flux bias. This guarantees that JPA 1 does not affect the measurements with JPA 2, and vice versa. The output signal is amplified at 4 K with a cryogenic high-electron-mobility transistor (HEMT) with gain  $G_H = 41$  dB. In a second amplification stage at room temperature, the signal is further amplified by an additional rf-amplifier, which is stabilized in temperature by a Peltier cooler. A vector network analyzer is used to characterize the JPA device parameters and to extract the dependence of the narrowband gain  $G_n$  on the JPA pump power for both JPAs. A narrowband coherent input signal is generated with a microwave source, and a heatable 30 dB attenuator at millikelvin temperatures with PID temperature control enables the generation of broadband thermal input states.

The measurement is realized with a heterodyne detection setup similar to the setup used in Ref. [S7–S9]. The amplified output signal is filtered with a 4.9 – 6.2 GHz bandpass filter and down-converted to 11 MHz with a local oscillator (LO). The resulting intermediate-frequency (IF) signal passes additional filters and a dc-block. Following this, analog-to-digital (ADC) converters, integrated in an Acqiris DC440 card, are used to digitize the signal. The digital signal is transmitted to a computer, where it is digitally down-converted (DDC) and filtered with a finite-impulse response (FIR) filter. The FIR filter determines the single-sided measurement bandwidth  $B$  of the setup. For our experiment, we use  $B/2\pi = 200$  kHz. After that, the quadrature moments  $\langle I^n Q^m \rangle$ ,  $n + m \leq 4$  with  $n, m \in \mathbb{N}$ , are calculated and averaged. The signal moments  $\langle (\hat{a}^\dagger)^n \hat{a}^m \rangle$  are determined with the reference-state reconstruction method [S7, S10]. Since this method relies on a vacuum state as a reference, we divide the 640  $\mu\text{s}$  acquisition window into two equal pulses, where the JPA pump signal is only switched on during the second pulse. This is realized with a data timing generator (DTG), which defines the modulation of the output of the JPA pump microwave sources and additionally provides the trigger pulse for the signal acquisition. The Acqiris card and the LO source are synchronized with a 10 MHz rubidium frequency standard and the pump sources are referenced to the LO with a 1 GHz reference signal.

As described in Ref. [S9], we assume that all reconstructed states are Gaussian, which means that only moments up to the second order are needed for the signal reconstruction [S11]. Moments of higher order are used to calculate the cumulants  $\langle\langle (\hat{a}^\dagger)^n \hat{a}^m \rangle\rangle$ , which are used as a benchmark for Gaussianity [S12].

## EXTRACTING THE QUANTUM EFFICIENCY FOR NARROWBAND SIGNALS

To measure the noise added by the amplification of broadband input signals, we vary the temperature  $T_{\text{att}}$  of the heatable 30 dB attenuator from 40 mK to 600 mK using a PID control architecture. We detect the quadrature moments  $\langle I^m Q^n \rangle$  with  $m, n \in \mathbb{N}_0$ ,  $m + n \leq 4$  from the digitized and filtered output signal. The detected power  $P(T_{\text{att}})$  is determined by the sum  $\langle I^2 \rangle + \langle Q^2 \rangle$  of the second order moments and follows a Planck curve [S13]

$$\begin{aligned}
 P(T_{\text{att}}) &= \frac{\langle I^2 \rangle + \langle Q^2 \rangle}{R} \\
 &= \frac{\kappa G_b \tilde{G}}{R} \left[ \frac{1}{2} \coth \left( \frac{\hbar \omega_s}{2k_B T_{\text{att}}} \right) + n_{f,b} \right],
 \end{aligned} \tag{S32}$$

where  $n_{f,b}$  is the total noise added by the amplification chain referred to the input,  $R = 50 \Omega$  is the line impedance,  $G_b$  is the broadband JPA gain,  $\tilde{G}$  is the gain of the HEMT and the remaining amplification chain and  $\kappa$  denotes the photon-number-conversion factor (PNCF). The gain dependence of  $n_{f,b}$  can be determined by repeating the temperature sweep for varying values of  $G_b$  and fitting a Planck curve to each of the results. To be able to experimentally control  $G_b$ , we use a vector network analyzer to measure the pump power dependence of the narrowband parametric gain  $G_n$ . We then expect  $G_b \simeq G_n + 3$  dB and measure Planck curves for expected  $G_b$  ranging from 6 dB to 27 dB in steps of 3 dB and fit Eq. (S32) to each experimental outcome. Since we measure with a two-pulsed scheme, where the JPA

pump signal is only switched on during the second pulse,  $G_b$  can be extracted directly from the measurement by calculating the ratio of the prefactors  $G_b \hat{G}$  of the Planck curves corresponding to the second pulse and first pulse. We calculate the broadband quantum efficiencies  $\eta_b = 1/(1 + 2n_{f,b})$  from the fit parameters. The error bars for the quantum efficiency are determined from the fit error  $\Delta n_{f,b}$  by error propagation.

### EXTRACTING THE QUANTUM EFFICIENCY FOR NARROWBAND SIGNALS

To calibrate the photon number in a coherent input signal, we switch the JPA pump off and tune the JPA resonance frequency out of the measurement bandwidth such that the JPA does not have any impact on the calibration procedure. We then perform Planck spectroscopy to determine the PNCF for the signal reconstruction point [S13]. The result of this calibration measurement is shown in Fig. S2(a). Following that, we vary the power  $P_{\text{coh}}$  of the coherent input signal and determine the photon number  $n_{\text{coh}}$  at the reconstruction point using the reference-state reconstruction method for each value of  $P_{\text{coh}}$ . This data can be linearly fitted according to

$$n_{\text{coh}}(P_{\text{coh}}) = k_1 P_{\text{coh}} + k_2, \quad (\text{S33})$$

where  $k_1$  and  $k_2$  are fitting parameters, as shown in Fig. S2(b). To measure the additive noise number, we tune the JPA into resonance and measure in the two-pulsed scheme. We vary the coherent input photon number  $n_{\text{in}}$  and measure the output photon number  $n_{\text{out}}$  for the case in which the JPA pump is switched off (first pulse). We repeat the measurement and detect the signal power  $n_{\text{JPA}}$  when the JPA pump is switched on. Both results are fitted linearly according to

$$n_{\text{out}} = k_3 n_{\text{in}} + k_4, \quad (\text{S34})$$

$$n_{\text{JPA}} = k_5 n_{\text{in}} + k_6 \quad (\text{S35})$$

with fitting constants  $k_3, k_4, k_5, k_6$ . From this, we extract the narrowband gain  $G_n = k_5/k_3$  and the total number of added noise photons  $n_{f,n} = k_6/G_n$ , referred to the input which allows us to calculate the narrowband quantum efficiency  $\eta_n$ . The error bars for  $\eta_n$  are determined from the fit by error propagation.

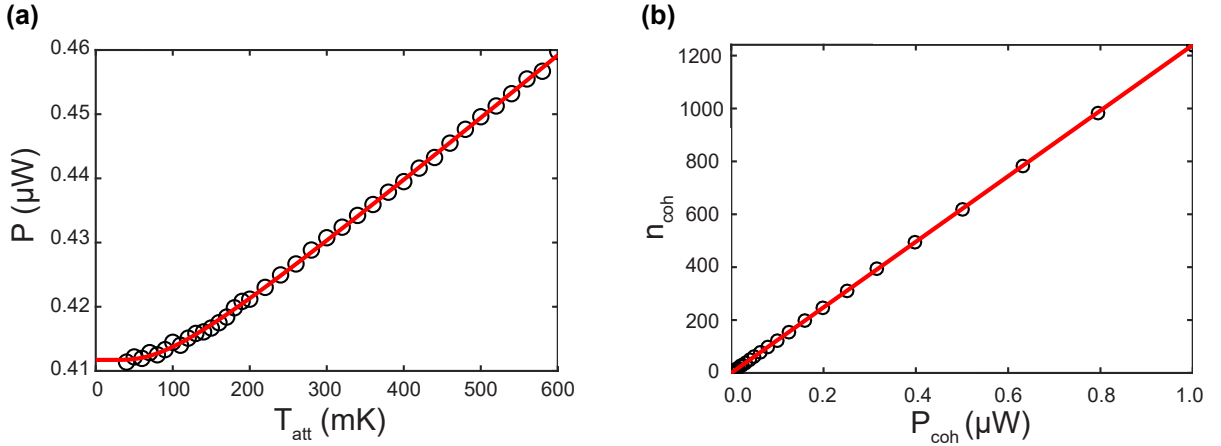

Figure S2. (a) Planck spectroscopy to determine the PNCF at the reconstruction point. Here,  $T_{\text{att}}$  denotes the temperature of the heatable attenuator and  $P$  is the power of the output signal, detected at the ADCs. (b) Photon number calibration in the coherent input signal at the reconstruction point. The coherent photon number  $n_{\text{coh}}$  is determined with the reference-state reconstruction method for each input power  $P_{\text{coh}}$ .

### GAIN DEPENDENCE OF PUMP INDUCED NOISE

We assume that the coherent pump signal  $\hat{A}(t)$  can be described as

$$\hat{A}(t) = (\alpha_0 + \hat{f}_p(t))e^{-i\omega_p t}, \quad (\text{S36})$$

where  $\alpha_0$  denotes the amplitude of the pump field which is assumed to be real and  $\hat{f}_p(t)$  denotes the bosonic operator for the superposed fluctuations. For the pump photon number operator  $\hat{n}_p(t)$  in the signal, we obtain

$$\hat{n}_p(t) = \hat{A}^\dagger(t)\hat{A}(t) = |\alpha_0|^2 + \alpha_0(\hat{f}_p(t) + \hat{f}_p^\dagger(t)) + \hat{f}_p^\dagger(t)\hat{f}_p(t). \quad (\text{S37})$$

Thus, the noise contribution  $\hat{n}_{f,p}$  in the pump line is given by  $\alpha_0(\hat{f}_p(t) + \hat{f}_p^\dagger(t)) + \hat{f}_p^\dagger(t)\hat{f}_p(t)$ . To find the corresponding noise spectral density, we calculate the autocorrelation function

$$\begin{aligned} \langle \hat{n}_{f,p}(t)\hat{n}_{f,p}(t-\tau) \rangle &= \alpha_0^2 \langle (\hat{f}_p(t) + \hat{f}_p^\dagger(t))(\hat{f}_p(t-\tau) + \hat{f}_p^\dagger(t-\tau)) \rangle + \alpha_0 \langle \hat{f}_p(t)\hat{f}_p^\dagger(t-\tau)\hat{f}_p(t-\tau) \rangle \\ &\quad + \alpha_0 \langle \hat{f}_p^\dagger(t)\hat{f}_p(t-\tau)\hat{f}_p(t-\tau) \rangle + \alpha_0 \langle \hat{f}_p^\dagger(t)\hat{f}_p(t)\hat{f}_p(t-\tau) \rangle + \alpha_0 \langle \hat{f}_p^\dagger(t)\hat{f}_p(t)\hat{f}_p^\dagger(t-\tau) \rangle \\ &\quad + \langle \hat{f}_p^\dagger(t)\hat{f}_p(t)\hat{f}_p^\dagger(t-\tau)\hat{f}_p(t-\tau) \rangle. \end{aligned} \quad (\text{S38})$$

We assume that the noise power spectrum is white, which implies

$$\begin{aligned} \langle \hat{n}_{f,p}(t)\hat{n}_{f,p}(t-\tau) \rangle &= \underbrace{\alpha_0^2 \langle (\hat{f}_p(t) + \hat{f}_p^\dagger(t))^2 \rangle}_{1} \delta(\tau) + \underbrace{\alpha_0 \langle \hat{f}_p^{\dagger 2}(t)\hat{f}_p(t) \rangle}_{2} \delta(\tau) \\ &\quad + \underbrace{\alpha_0 \langle \hat{f}_p^\dagger(t)\hat{f}_p^2(t) \rangle}_{3} \delta(\tau) + \underbrace{\alpha_0 \langle \hat{f}_p^\dagger(t)\hat{f}_p(t)\hat{f}_p^\dagger(t) \rangle}_{4} \delta(\tau) \\ &\quad + \underbrace{\langle \hat{f}_p^\dagger(t)\hat{f}_p(t)\hat{f}_p^\dagger(t)\hat{f}_p(t) \rangle}_{5} \delta(\tau), \end{aligned} \quad (\text{S39})$$

where  $\delta(\tau)$  denotes the Dirac delta function. The contributions 2, 3 and 4 vanish since they contain odd moments of  $\hat{f}_p(t)$  and the probability distribution for  $\hat{f}_p(t)$  is assumed to be centralized around zero, which leads to

$$\langle \hat{n}_{f,p}(t)\hat{n}_{f,p}(t-\tau) \rangle = \{ \alpha_0^2 \langle (\hat{f}_p(t) + \hat{f}_p^\dagger(t))^2 \rangle + \hat{f}_p^\dagger(t)\hat{f}_p(t)\hat{f}_p^\dagger(t)\hat{f}_p(t) \} \delta(\tau). \quad (\text{S40})$$

Using the bosonic commutation relations

$$[\hat{f}_p(t), \hat{f}_p^\dagger(t)] = 1, \quad (\text{S41})$$

we can rewrite Eq. (S40) in terms of normally ordered moments

$$\langle \hat{n}_{f,p}(t)\hat{n}_{f,p}(t-\tau) \rangle = \{ \alpha_0^2 (\langle \hat{f}_p(t)^2 \rangle + \langle \hat{f}_p^\dagger(t)^2 \rangle + 2\langle \hat{f}_p^\dagger(t)\hat{f}_p(t) \rangle + 1) + \langle \hat{f}_p(t)^{\dagger 2}\hat{f}_p(t)^2 \rangle + \langle \hat{f}_p(t)^\dagger \hat{f}_p(t) \rangle \} \delta(\tau). \quad (\text{S42})$$

We apply the Wiener-Khinchine theorem to get the variance  $\sigma_p^2$  of the noise power [S14, S15]

$$\sigma_p^2 = \int_{-\infty}^{\infty} e^{i\omega\tau} \langle n_{f,p}(t)n_{f,p}(t-\tau) \rangle d\tau = \alpha_0^2 (\langle \hat{f}_p(t)^2 \rangle + \langle \hat{f}_p^\dagger(t)^2 \rangle + 2\langle \hat{f}_p^\dagger(t)\hat{f}_p(t) \rangle + 1) + \langle \hat{f}_p(t)^{\dagger 2}\hat{f}_p(t)^2 \rangle + \langle \hat{f}_p(t)^\dagger \hat{f}_p(t) \rangle. \quad (\text{S43})$$

We assume that  $\hat{f}_p$  obeys thermal statistics, which implies

$$\langle \hat{f}_p^\dagger(t)^n \hat{f}_p(t)^m \rangle = n! \delta_{nm} n_{\text{th}}^n, \quad (\text{S44})$$

where  $n_{\text{th}}$  denotes the average thermal photon number. Furthermore, we set  $\alpha_0^2 = n_p$ , where  $n_p$  is the expectation value for the coherent photons in the pump signal. Thus, we find

$$\sigma_p^2 = n_p(2n_{\text{th}} + 1) + 2n_{\text{th}}^2 + n_{\text{th}}. \quad (\text{S45})$$

In the next step, we need to gain knowledge about the dependence of the parametric gain on  $n_p$ . Figure S3 shows the detected narrowband gain  $G_n$  for varying pump power  $P_p$ . The result can be exponentially fitted, as illustrated by the solid orange line. Since  $n_p \propto P_p$ , we can make the ansatz

$$G_n(n_p) = C e^{a n_p}, \quad (\text{S46})$$

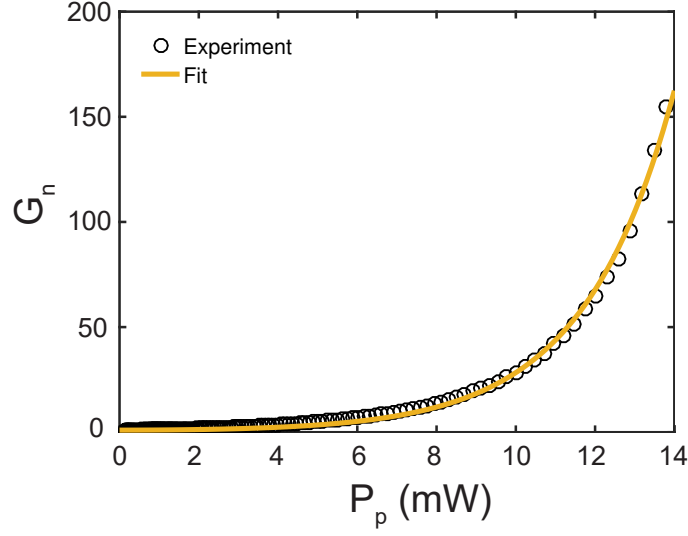

Figure S3. Measured dependence of the parametric gain  $G_n$  on the applied pump power  $P_p$ . The orange line shows an exponential fit of the data.

with yet unspecified constants  $C$  and  $a$ . From  $n_p = 1/a \ln(G_n/C)$ , we obtain the gain dependence of the fluctuations in the pump line

$$\sigma_p^2 = \frac{(2n_{th} + 1)}{a} \ln \left( \frac{G_n}{C} \right) + 2n_{th}^2 + n_{th}. \quad (S47)$$

The fluctuations in the pump photon number translate to fluctuations in  $G_n$ . These fluctuations in  $G_n(t)$  are characterized by the variance

$$\text{Var}(G_n(t)) = \langle G_n^2(t) \rangle - G_n^2. \quad (S48)$$

We assume that the noise  $n_J$  added to the amplified signal is proportional to the fluctuations in the parametric gain. We refer the fluctuations to the input by dividing by the squared average gain  $G_n^2$

$$n_J \propto \frac{\text{Var}(G_n(t))}{G_n^2} = \frac{\langle G_n(t)^2 \rangle}{G_n^2} - 1. \quad (S49)$$

For the relative gain fluctuations, we find

$$\frac{\langle G_n(t)^2 \rangle}{G_n^2} = \langle e^{2a\zeta(t)} \rangle \quad (S50)$$

with  $\zeta(t) = n_p(t) - n_p$ . We assume that the fluctuations  $\zeta(t)$  can be described by a centralized normal distribution with variance  $\sigma_p^2$ . Thus, we find for the moments with  $n > 2$

$$\langle \zeta(t)^n \rangle = \sigma_p^n \frac{2^{n/2} \Gamma(\frac{n+1}{2})}{\sqrt{\pi}} = \begin{cases} 0 & \text{if } n \text{ is odd} \\ \sigma_p^n (n-1)!! & \text{if } n \text{ is even} \end{cases}. \quad (S51)$$

Thus, we find

$$\langle e^{2a\zeta(t)} \rangle = \sum_{n=0}^{\infty} \frac{(2a)^n}{n!} \langle \zeta(t)^n \rangle = 1 + \sum_{n=1}^{\infty} \frac{(2a\sigma_p)^{2n} (2n-1)!!}{(2n)!} = e^{2a^2\sigma_p^2}. \quad (S52)$$

Using this expression, we find from Eq. (S47)

$$n_J \propto G_n^\epsilon - 1 \simeq (G_n - 1)^\epsilon \quad (S53)$$

and  $\epsilon = 2a(2n_{th} + 1)$ .

## FITTING THE MEASURED QUANTUM EFFICIENCIES

### Fitting the measured quantum efficiencies

The total additive noise  $n_f$ , referred to the input of the amplification chain, can be related to the JPA noise  $n_J$  and the HEMT noise  $n_H$  with the Friis equation [S16]

$$n_f = n_J + \frac{n_H}{G}, \quad (\text{S54})$$

where  $G$  denotes the JPA gain (either narrowband or broadband). Thus, we can express the quantum efficiency  $\eta$  as

$$\eta = \frac{G}{G + 2Gn_J + 2n_H}. \quad (\text{S55})$$

The JPA noise  $n_J$  is dependent on  $G$ . For  $G = 1$ , i.e. when the JPA is switched off, we expect  $n_J = 0$ . We assume that the gain-dependent noise  $n_{J,b}(G)$  for amplification of broadband signals mainly results from pump induced fluctuations and fit the measured quantum efficiencies for the broadband case using

$$\eta_b(G_b) = \frac{G_b}{G_b + 2G_b n'_{J,b}(G_b - 1)^{\epsilon_b} + 2n_H}, \quad (\text{S56})$$

where we treat  $n'_{J,b}$  and  $\epsilon_b$  as fitting parameters and insert  $n_H = 11.3$ . For the narrowband quantum efficiency  $\eta_n$ , we assume that the idler mode adds additional vacuum fluctuations to the signal. Thus, we assume for the noise photons

$$n_{J,n}(G_n) = \underbrace{n'_{J,n}(G_n - 1)^{\epsilon_n}}_{\text{Pump-induced}} + \underbrace{\frac{1}{2} \left( 1 - \frac{1}{G_n} \right)}_{\text{SQL}}, \quad (\text{S57})$$

implying that we use

$$\eta_n(G_n) = \frac{G_n}{2G_n - 1 + 2G_n n'_{J,n}(G_n - 1)^{\epsilon_n} + 2n_H} \quad (\text{S58})$$

as a fit function for this case, where we treat  $n'_{J,n}$  and  $\epsilon_n$  as fit parameters. The fit parameters for the broadband and narrowband quantum efficiencies are listed in Tab. S2.

Table S2. Fit parameters corresponding to the measured broadband and narrowband quantum efficiencies of JPA 1 and JPA 2 in Fig. 4 of the main text.

| Fit parameter | $n'_{J,b}$             | $\epsilon_b$ | $n'_{J,n}$ | $\epsilon_n$ |
|---------------|------------------------|--------------|------------|--------------|
| JPA 1         | $6.0342 \cdot 10^{-6}$ | 2.5375       | 0.4552     | 0.1312       |
| JPA 2         | $8.4789 \cdot 10^{-5}$ | 1.524        | 0.5326     | 0.0591       |

We acknowledge support by the German Research Foundation through the Munich Center for Quantum Science and Technology (MCQST), Elite Network of Bavaria through the program ExQM, EU Flagship project QMiCS (Grant No. 820505).

---

\* michael.renger@wmi.badw.de

† kirill.fedorov@wmi.badw.de

- [S1] C. M. Caves, Phys. Rev. D **26**, 1817 (1982).
- [S2] A. Roy and M. Devoret, C R Phys **17**, 740 (2016).
- [S3] T. Yamamoto, K. Inomata, M. Watanabe, K. Matsuba, T. Miyazaki, W. D. Oliver, Y. Nakamura, and J. S. Tsai, Appl. Phys. Lett. **93**, 042510 (2008).
- [S4] T. Yamamoto, K. Koshino, and Y. Nakamura, *Principles and Methods of Quantum Information Technologies*, edited by Y. Yamamoto and K. Semba (Springer, 2016) Chap. 23, pp. 495–513.
- [S5] L. Zhong, E. P. Menzel, R. D. Candia, P. Eder, M. Ihmig, A. Baust, M. Haeberlein, E. Hoffmann, K. Inomata, T. Yamamoto, Y. Nakamura, E. Solano, F. Deppe, A. Marx, and R. Gross, New J. Phys. **15**, 125013 (2013).
- [S6] S. Pogorzalek, K. G. Fedorov, L. Zhong, J. Goetz, F. Wulschner, M. Fischer, P. Eder, E. Xie, K. Inomata, T. Yamamoto, Y. Nakamura, A. Marx, F. Deppe, and R. Gross, Phys. Rev. Appl. **8**, 024012 (2017).
- [S7] K. G. Fedorov, S. Pogorzalek, U. Las Heras, M. Sanz, P. Yard, P. Eder, M. Fischer, J. Goetz, E. Xie, K. Inomata, Y. Nakamura, R. Di Candia, E. Solano, A. Marx, F. Deppe, and R. Gross, Sci. Rep. **8**, 6416 (2018).
- [S8] E. P. Menzel, F. Deppe, M. Mariani, M. A. Araque Caballero, A. Baust, T. Niemczyk, E. Hoffmann, A. Marx, E. Solano, and R. Gross, Phys. Rev. Lett. **105**, 100401 (2010).
- [S9] S. Pogorzalek, K. G. Fedorov, M. Xu, A. Parra-Rodriguez, M. Sanz, M. Fischer, E. Xie, K. Inomata, Y. Nakamura, E. Solano, A. Marx, F. Deppe, and R. Gross, Nat. Commun. **10**, 2604 (2019).
- [S10] C. Eichler, D. Bozyigit, C. Lang, L. Steffen, J. Fink, and A. Wallraff, Phys. Rev. Lett. **106**, 220503 (2011).
- [S11] S. L. Braunstein and P. van Loock, Rev. Mod. Phys. **77**, 513 (2005).
- [S12] E. P. Menzel, R. Di Candia, F. Deppe, P. Eder, L. Zhong, M. Ihmig, M. Haeberlein, A. Baust, E. Hoffmann, D. Ballester, K. Inomata, T. Yamamoto, Y. Nakamura, E. Solano, A. Marx, and R. Gross, Phys. Rev. Lett. **109**, 250502 (2012).
- [S13] M. Mariani, E. P. Menzel, F. Deppe, M. A. Araque Caballero, A. Baust, T. Niemczyk, E. Hoffmann, E. Solano, A. Marx, and R. Gross, Phys. Rev. Lett. **105**, 133601 (2010).
- [S14] P. Kylemark, M. Karlsson, and P. A. Andrekson, IEEE Photonics Technol. Lett. **18**, 1255 (2006).
- [S15] N. A. Olsson, J. Lightwave Technol. **7**, 1071 (1989).
- [S16] D. M. Pozar, *Microwave engineering*, 4th ed. (Wiley, Hoboken, 2012).
